# Supplementary material for: Embedding based on function approximation for large scale image search
Source: arXiv:1605.06914 source file (2017-04-04)
Supplement: Supplementary file 1 [file appendix.tex]

\appendix
\section{Appendix}
\subsection{Proof of Lemma~\ref{lemma_1}}
\label{proof_lemma_1}
%First, let us introduce and proof following lemma
%\begin{lemma}
%If $\R^d \to \R$ is of class of $C^{k+1}$ and $\nabla^k f(\x)$ is Lipschitz continuous, then exist $M$ such that $|\partial^{\alpha}f(\x)| \le M$ for $\x\in R^d$ and $|\alpha| = k+1$
%\end{lemma}
%\textbf{Proof:} 
Because $\nabla^k f(\x)$ is Lipschitz continuous with constant $M>0$, we have $\norm{\nabla^{k+1} f(\x)}_{2} \le M$. So for $| \alpha | = k+1$, we have $\vert \partial^{\alpha} f( \x )\vert \le \norm{\nabla^{k+1} f(\x)}_{2} \le M$.
%Because $\nabla^k f(\x)$ is Lipschitz continuous with constant $M$, we have $\norm{\nabla^{k+1} f(\x)}_{2} \le M$. This means that $\vert \partial^{\alpha} f( \x )\vert \le M$ for $| \alpha | = k+1$

We have
\begin{eqnarray}
{} & & \left| f(\x) - \sum_{j=1}^{n} \gamma_{\v_j}(\x)  \sum_{ | \alpha | \le k} \frac{\partial^{\alpha} f(\v_j)}{\alpha!} \left( \x -  \v_j \right)^\alpha \right|  \nonumber \\
{} & = & \left| \sum_{j=1}^{n} \gamma_{\v_j}(\x) \left( f(\x) -   \sum_{ | \alpha | \le k} \frac{\partial^{\alpha} f(\v_j)}{\alpha!} \left( \x -  \v_j \right)^\alpha \right) \right| \nonumber \\
{} & \le &  \sum_{j=1}^{n} \left| \gamma_{\v_j}(\x) \left( f(\x) -   \sum_{ | \alpha | \le k} \frac{\partial^{\alpha} f(\v_j)}{\alpha!} \left( \x -  \v_j \right)^\alpha \right) \right| \nonumber \\
{} & = &  \sum_{j=1}^{n} \left| \gamma_{\v_j}(\x) \right| \left|   R_{\v_j, k}(\x - \v_j)  \right| \nonumber \\
{} &\le& \frac{M}{(k+1)!} \sum_{j=1}^{n} \left|\gamma_{\v_j}(\x) \right| \norm{\x-\v_j}_{1}^{k+1} \nonumber .
\end{eqnarray}
where the last inequation comes from corollary~\ref{bound_remainder}.
\subsection{Gradient and Hessian w.r.t. $\gamma_i, \C$ of objective function $Q(\Gamma, \C)$ \protect \footnotemark}
%\footnotetext{The partial derivatives $\partial(Q)/\partial \gamma_{i_k}$ and $\partial(Q)/\partial \v_{j_k}$ % and $\partial^2(Q)/\partial \v_{i_k}\partial \v_{i_h}$ do not exist at some points (i.e. at $\gamma_{i_k} = 0$ and at $\v_{j_k} - \x_{i_k} = 0$, respectively). We found, however, the Newton's method and the trust-region method with the provided derivatives works well in practice.}
\footnotetext{Theoretically, the partial derivatives $\partial(Q)/\partial \gamma_{i_k}$ and $\partial(Q)/\partial \v_{j_k}$ do not exist at some points. We found, however, the Newton's method and the trust-region method with the provided derivatives work well in practice.}
We have the objective function
\begin{eqnarray}
%\label{eq:objective}
Q(\Gamma, \C) &=& \sum_{i = 1}^{m} \left[ \norm{\x_i - \C\gamma_i}_{2}^2 + \mu \sum_{j=1}^{n} |\gamma_{i_j}| \norm{\x_i - \v_j}_{1}^3 \right] \nonumber 
\end{eqnarray}

\label{app:derivative}
\subsubsection{Gradient and Hessian w.r.t. $\gamma_i$}
Let $\a = \left[\norm{\x_i - \v_1}_1^3,\norm{\x_i - \v_2}_1^3, \dots, \norm{\x_i - \v_n}_1^3\right]^T$, we have
\begin{eqnarray}
\nabla Q(\gamma_i) &=& 2\C^T(\C\gamma_i - \x_i) + \mu\ sign(\gamma_i)\odot \a \\ %\footnotemark
\nabla^2 Q(\gamma_i) &=& 2\C^T\C
\end{eqnarray}
where $sign(\gamma_i) = \left[ sign(\gamma_{i_1}), sign(\gamma_{i_2}),\dots, sign(\gamma_{i_n}) \right]^T$ and $\odot$ denotes Hadamard product.

\subsubsection{Derivative and Hessian w.r.t. $\C$}
Let $R = \sum_{i = 1}^{m} \norm{\x_i - \C\gamma_i}_{2}^2 = \norm{\X-\C\Gamma}_{2}^2$, we have 
\begin{equation}
\nabla R(\C)  = 2(\C\Gamma - \X)\Gamma^T
\end{equation}

Let $L =  \sum_{j=1}^{n} \sum_{i=1}^{m} |\gamma_{i_j}| \norm{\x_i - \v_j}_{1}^3$ and
let $\d_j = \nabla L(\v_j)= 3\sum_{i=1}^{m} |\gamma_{i_j}| \norm{\v_j - \x_i}_{1}^2 sign (\v_j -\x_i) $, we have
\begin{equation}
\nabla L(\C) = \left[ \d_1, \dots, \d_j, \dots, \d_n \right]
\end{equation}
Finally, we get
\begin{equation}
\nabla Q(\C) = \nabla R(\C) + \mu\nabla L(\C)
\end{equation}

Let $u_j = \sum_{i=1}^{m}\gamma_{i_j}^2$: sum of square of coefficients corresponding to base $\v_j$ of all data points $\x$; let  $\A_{jj} = 2u_j\mathbf{I}_{d\times d} \in \R^{d \times d}, j = 1,\dots, n$, we have
\begin{equation}
\nabla^2 R(\C) =
\left( \begin{array}{cccc}
\A_{11} & \0_{d\times d} & \ldots & \0_{d\times d}\\
\0_{d\times d} & \A_{22} & \ldots & \0_{d\times d} \\
\vdots & \vdots & \ddots & \0_{d\times d}\\
\0_{d\times d} & \0_{d\times d}  & \ldots &  \A_{nn}
\end{array} \right)
\end{equation}
where $\0_{d \times d}$ is matrix having size of $d\times d$ and zero elements.\\

Let $\B_{jj} = \nabla^2 L (\v_j) \in \R^{d \times d}$ be Hessian of $L$ w.r.t. base $\v_j$, $j = 1,\dots,n$, we have
\begin{equation}
\B_{jj} = 
\left( \begin{array}{cccc}
\frac{\partial^2 L}{\partial \v_{j_1}\partial \v_{j_1}} & \frac{\partial^2 L}{\partial \v_{j_1}\partial \v_{j_2}} & \ldots & \frac{\partial^2 L}{\partial \v_{j_1}\partial \v_{j_d}}	\\
\frac{\partial^2 L}{\partial \v_{j_2}\partial \v_{j_1}} & \frac{\partial^2 L}{\partial \v_{j_2}\partial \v_{j_2}} & \ldots & \frac{\partial^2 L}{\partial \v_{j_2}\partial \v_{j_d}} \\
\vdots & \vdots & \ddots & \vdots
\\
\frac{\partial^2 L}{\partial \v_{j_d}\partial \v_{j_1}} & \frac{\partial^2 L}{\partial \v_{j_d}\partial \v_{j_2}}  & \ldots &  \frac{\partial^2 L}{\partial \v_{j_d}\partial \v_{j_d}}
\end{array} \right)
%\B_{jj} = 
%\left( \begin{array}{ccccc}
%\frac{\partial^2 L}{\partial \v_{j_1}\partial \v_{j_1}} & \ldots & \frac{\partial^2 L}{\partial \v_{j_1}\partial \v_{j_h}} & \ldots & \frac{\partial^2 L}{\partial \v_{j_1}\partial \v_{j_d}}	\\
%\vdots & \ddots & \vdots & \vdots &  \vdots \\
%\frac{\partial^2 L}{\partial \v_{j_k}\partial \v_{j_1}} & \ldots & \frac{\partial^2 L}{\partial \v_{j_k}\partial \v_{j_h}} & \ldots & \frac{\partial^2 L}{\partial \v_{j_k}\partial \v_{j_d}} \\
%\vdots & \vdots & \vdots & \ddots & \vdots \\
%\frac{\partial^2 L}{\partial \v_{j_d}\partial \v_{j_1}} & \ldots & \frac{\partial^2 L}{\partial \v_{j_d}\partial \v_{j_h}}  & \ldots &  \frac{\partial^2 L}{\partial \v_{j_d}\partial \v_{j_d}}
%\end{array} \right)
\end{equation}

For $k = 1,\dots, d$; $h = 1,\dots,d$; if $k = h$ then
\begin{displaymath}
\frac{\partial^2 L}{\partial \v_{j_k}\partial \v_{j_h}} = 6\sum_{i=1}^{m}|\gamma_{i_j}| \norm{\v_j-\x_i}_{1} \left(sign(\v_{j_k}-\x_{i_k}) \right)^2
\end{displaymath}
If $k \neq h$ then 
\begin{eqnarray}
\frac{\partial^2 L}{\partial \v_{j_k}\partial \v_{j_h}} \hspace{20em}  && {}  \nonumber \\
=6\sum_{i=1}^{m}|\gamma_{i_j}|  \norm{\v_j-\x_i}_{1} sign(\v_{j_k}-\x_{i_k}) sign(\v_{j_h}-\x_{i_h}) &&{} \nonumber
\end{eqnarray}
%\begin{displaymath}
%\frac{\partial^2 L}{\partial \v_{j_k}\partial \v_{j_h}} = \left\{ \begin{array}{ll}
%3\mu\sum_{i=1}^{m}|\gamma_{i_j}| \left( \norm{\v_j-\x_i}_{2} + \frac{(\v_{j_k}-\x_{i_k})^2}{\norm{\v_j-\x_i}_{2}} \right) & if\ k = h\\
%3\mu\sum_{i=1}^{m}|\gamma_{i_j}|  \frac{(\v_{j_k}-\x_{i_k})(\v_{j_h}-\x_{i_h})}{\norm{\v_j-\x_i}_{2}}  & if\ k \neq h\\
%\end{array} \right.
%\end{displaymath}
%$k = 1,\dots, d$; $h = 1,\dots,d$.

We have
\begin{equation}
\nabla^2 L(\C) =
\left( \begin{array}{cccc}
\B_{11} & \0_{d\times d} & \ldots & \0_{d\times d}\\
\0_{d\times d} & \B_{22} & \ldots & \0_{d\times d} \\
\vdots & \vdots & \ddots & \0_{d\times d}\\
\0_{d\times d} & \0_{d\times d}  & \ldots &  \B_{nn}
\end{array} \right)
\end{equation}
Finally, we get 
\begin{equation}
\nabla^2 Q(\C) = \nabla^2 R(\C) + \mu\nabla^2 L(\C)
\end{equation}
